# Supplementary material for: Collapsing the bounded width hierarchy for infinite-domain CSPs: when symmetries are enough
Source: arXiv:2102.07531 source file (2024-07-16)
Supplement: Supplementary file 1 [file appendix.tex]

\section{Bounded width}

The following lemma gives an overview of conditions characterizing relational structures with bounded width that are used in several proofs later.

\begin{lemma}\label{lemma:characterization-bwidth}
Let $\rel A$ be a finite relational structure and let $\rel B$ be its core. The following are equivalent.

\begin{enumerate}
    \item $\rel A$ has bounded width.
    \item $\rel A$ has relational width $(2,3)$.
    \item The class of structures $\{\rel X\mid \rel X\not\rightarrow\rel A\}$ is definable by a Datalog program.
    \item $\Pol(\rel A)$ does not admit a minion homomorphism to an affine clone.
    \item $\Pol(\rel B)$ is not equationally affine.
    \item $\Pol(\rel B)$ contains WNU operations of all arities $n\geq 3$.
\end{enumerate}
\end{lemma}

\begin{proof}
The equivalence of (1) and (2) was proven in~\cite{BartoCollapse}, the equivalence of (1) and (3) follows from definition. The implication from (1) to (5) is easy, (5) implies (6) by \cite{MarotiMcKenzie} (this stronger  version is attributed to E.\ Kiss in~\cite[Theorem 2.8]{Kozik2015}, a different proof can be found in~\cite{StrongSubalgebras}) and (6) implies (2) by Theorem~\ref{thm:bwidth-finite}. Finally, the equivalence of (1) and (4) follows from the equivalence of (1) and (5) combined with~\cite{wonderland}.
\end{proof}

For $\omega$-categorical relational structures, only items (1) and (3) in the theorem above are equivalent in general. For the structures that are considered in the presented article, the criterion for bounded width will be the non-existence of a uniformly continuous minion homomorphism from the polymorphism clone of the structure to an affine clone. By~\cite[Theorem 1.8]{wonderland}, given an at most countable $\omega$-categorical structure $\rel A$ and a finite structure $\rel B$, the existence of a uniformly continuous minion homomorphism from $\Pol(\rel A)$ to $\Pol(\rel B)$ is equivalent to $\rel B$ having a \emph{pp-construction} in $\rel A$. We say that $\rel B$ has a pp-construction in $\rel A$ if $\rel B$ is homomorphically equivalent to a structure with domain $A^n$, where $n\geq 1$, whose relations are pp-definable in $\rel A$ (a $k$-ary relation on $A^n$ is regarded as a $kn$-ary relation on $A$). The expansion of a core structure by singleton relations is a (non-trivial) example of a pp-construction.

Let $p\geq 2$ be prime and let $R_0$ and $R_1$ be the relations defined by $\{(x,y,z)\in\rel Z_p\mid x+y+z=i\bmod p\}$ for $i\in\{0,1\}$. For an arbitrary $\omega$-categorical structure $\rel A$, it is known that the existence of a uniformly continuous minion homomorphism from $\Pol(\rel A)$ to an affine clone is equivalent to the existence of a $p$ such that the relational structure $(\rel Z_p; R_0,R_1)$ has a pp-construction in $\rel A$. Moreover, if $\Pol(\rel A)$ does not have a uniformly continuous minion homomorphism to an affine clone, $\rel A$ does not have bounded width by results from~\cite{LaroseZadori, wonderland}. It is also known that if $\rel A$ is an $\omega$-categorical model-complete core, then $\Pol(\rel A)^{\canonical}$ is either equationally affine, or it contains pseudo-WNU operations modulo $\overline{\Aut(\rel A)}$ of all arities $n \geq 3$ (see~\cite{BPP-projective-homomorphisms, SmoothApproximations} for the lift of the corresponding result from the finite).
